# Supplementary material for: Efficient Replay Memory Architectures in Multi-Agent Reinforcement Learning for Traffic Congestion Control
Source: arXiv:2407.16034 source file (2024-07-22)
Supplement: Supplementary file 1 [file appendix.tex]

%\newpage
% \appendix
% \onecolumn
\section{Dual-Memory Hyperparameter Designs}\label{app:dual_memory_hyperparameter}
\begin{figure}[H]
\centering
 \centering
    \begin{subfigure}
    \centering
    \includegraphics[width=0.45\textwidth]{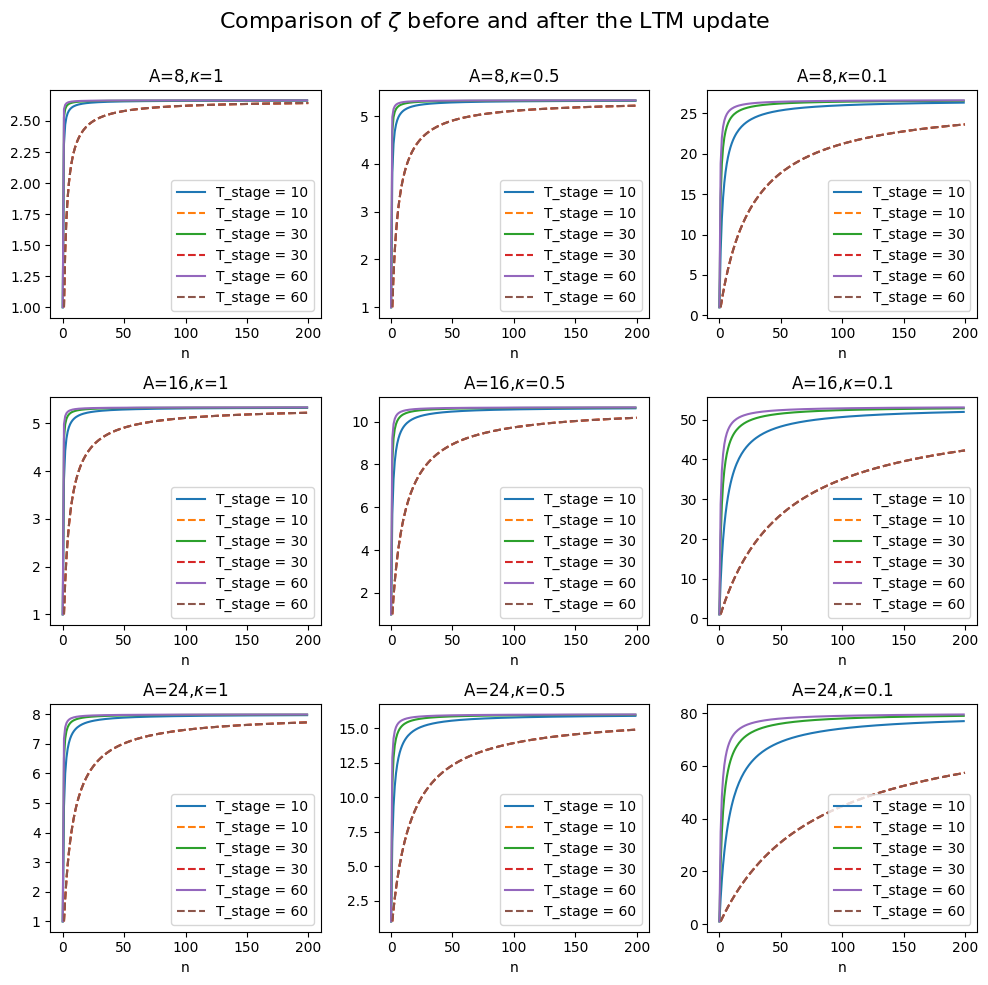}
    % \caption{Worst-case scenario as mentioned in Section \ref{sec:worst_case_traj}.}
    \label{fig:memory_size comparison_worst}
    \end{subfigure}
    \hfill
    \begin{subfigure}
            \centering
    \includegraphics[width=0.45\textwidth]{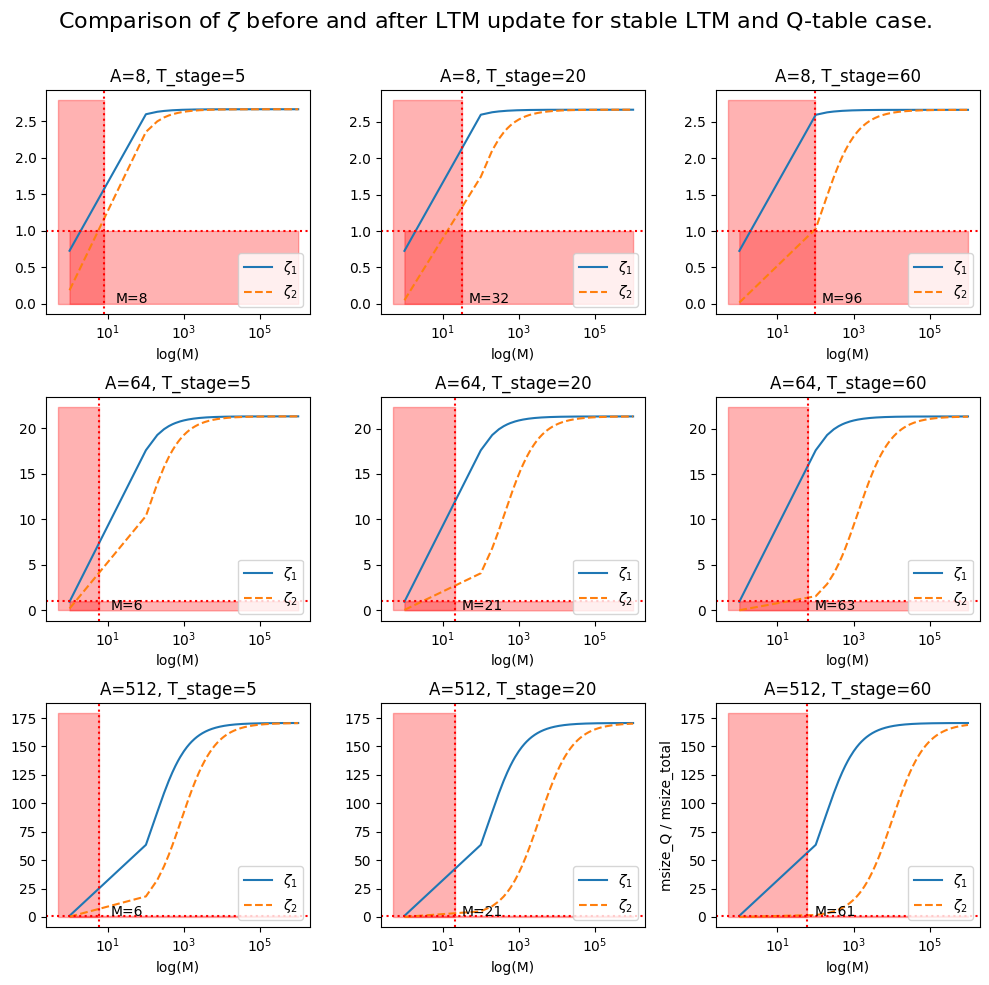}
    % \caption{Best-case scenario as mentioned in Section \ref{sec:best_case_traj}. }
    \label{fig:memory_size comparison_best}
    \end{subfigure}
    \caption{Memory size comparisons with different system parameters. Solid lines are from $\zeta_1$ and dashed from $\zeta_2$. The worst-case scenario (top), and best-case scenario (bottom) as mentioned in Section \ref{sec:analysis}. From both figures, it can be seen that the dual-memory architecture benefits from large action space and the $\zeta$ increases proportionally with it. The LTM staging period is also informed by the size of the unique state space. The shaded regions in the bottom figure show areas where the dual memory architecture is not as memory efficient as the replay buffer in the best-trajectory scenario (\cref{lem:best_traj})}
    \label{fig:memory_size comparison}.  
\end{figure}

%%%%%%%%%%%%%%%%%%%%%%%%%%%%%%%%%%%%%%%%%%%%%%%%%%%%%%%%%%%%%%%%%%%%%%%%%%%%%%%

% \section{Intersection Model}\label{app:3x3}
% \begin{figure}[ht]
%         \centering
%         \includegraphics[width=0.45\textwidth]{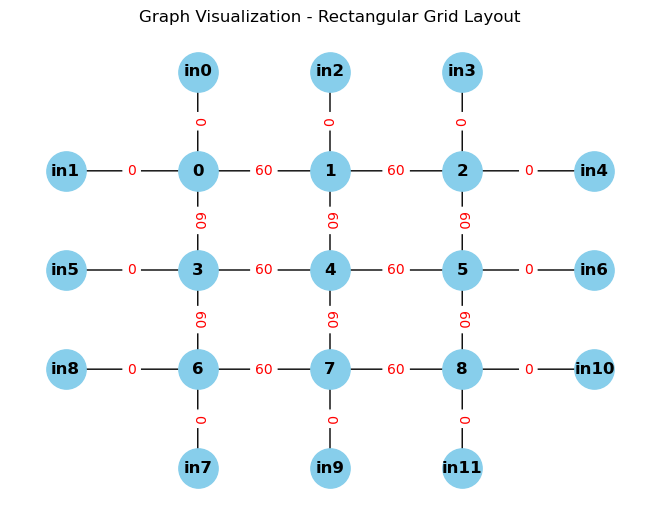}
%         \caption{A visualization of the $3\times 3$ intersection network used for our experiments.}\label{fig:sample_graph_structure}
% \end{figure}

%%%%%%%%%%%%%%%%%%%%%%%%%%%%%%%%%%%%%%%%%%%%%%%%%%%%%%%%%%%%%%%%%%%%%%%%%%%%%%%

\section{Memory Size Comparisons per Intersection}\label{app:mem_size_comparisons}

\begin{figure}[H]
\centering 
    \includegraphics[width = 0.5\textwidth]{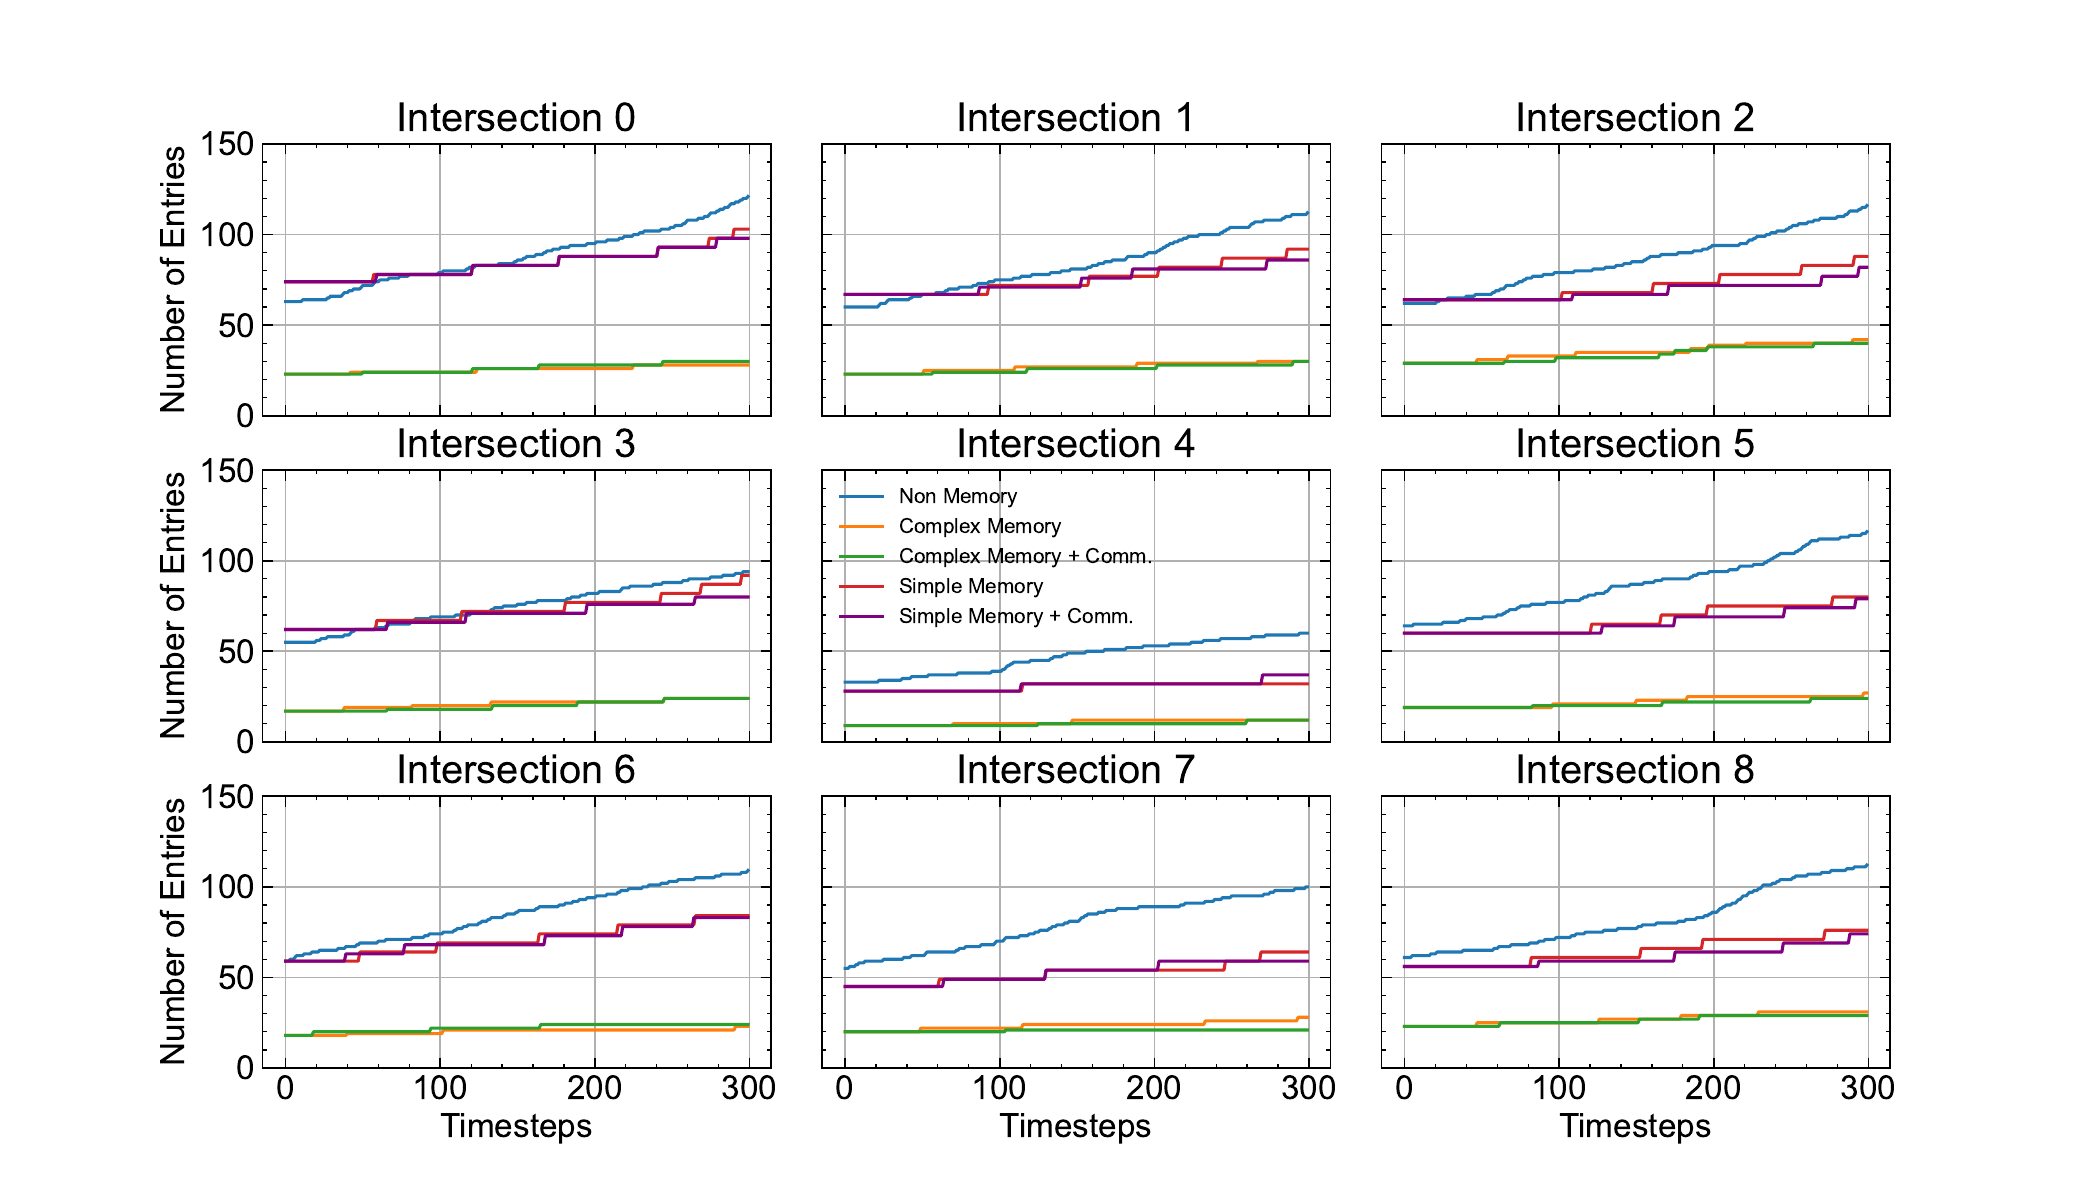}
    \caption{Memory table growth over time for each intersection in our $3\times 3$ grid network. 
    For non-memory, the number of Q-table entries are shown instead.
    We observe that each intersection follows relatively the same trend as the averaged case (\cref{fig:memory_entry_avg}).
    }
    \label{fig:q_table_size}
\end{figure}
